# Supplementary material for: Assigning Agents to Increase Network-Based Neighborhood Diversity
Source: arXiv:2301.02876 source file (2024-03-29)
Supplement: Supplementary file 1 [file additional_results.tex]

\subsubsection*{Polynomial Time Algorithm for Grids}
For the sake of convenience, we can represent an $a\times b$ grid graph using a rectangular board with $a$ rows and $b$ columns, where each cell corresponds to a node and adjacent cells correspond to adjacent nodes. We also place one agent into each cell of the board, which corresponds to mapping one agent onto each node of the graph. Thus, on the board, $\IoAgent{}$ is simply the number of cells that are adjacent to at least one different-type cell (just like with nodes, we define the type of a cell as the type of its corresponding agent).

Now, define a {\em fragment} to be any fragment of an X-pentomino, and we say a fragment is {\em proper} if it contains at least two cells. Moreover, when agents are placed onto the board, we define a fragment to be {\em self-integrated} if every cell in the fragment is adjacent to a different-type cell in the same fragment. Finally, in a placement, we define the integrated area to be the set of all cells which are integrated. We now prove an important lemma:

Lemma: In any placement, the integrated area can be tiled with self-integrated proper fragments.

Proof: First, it is easy to see that the integrated area can be tiled with self-integrating (not necessarily proper) fragments, as such: we iterate through the set of integrated type-1 cells, and for each such cell, we form a block consisting of the type-1 cell and all its neighboring type-2 cells that aren't already in a block. This way, these blocks tile the integrated area, and each block is a self-integrated fragment. To show that the integrated area can be covered with {\em proper} fragments, it suffices to show that for any integrated single-cell fragment, we can merge it with an adjacent fragment and then split the combined block to create two self-integrated proper fragments. 

To do this, WLOG suppose we are given a fragment $F_1$ consisting of a single integrated type-1 cell; then, we consider the fragment to which an adjacent type-2 cell belongs, and denote it as $F_2$. If $F_2$ only has one type-2 cell, then we can simply combine $F_1$ and $F_2$ to create a self-integrated proper fragment. We now consider all possible cases where $F_2$ has 2, 3, or 4 type-2 cells: [Insert diagrams here; there are 13 total configurations] End lemma.

Now, let $T$ be the maximum number of X-pentominos that can fit on the board, and let $U$ be the minimum number of fragments needed to fully tile the board. Also, suppose that there are $p$ type-1 cell and $q$ type-2 cell, and WLOG assume that $p\le q$. I claim that for $p\le T$, we have $\max(\IoAgent{})=5k$, and for $p\ge U$, we have $\max(\IoAgent{})=n$. 

First we prove that if $p\le T$, then $\max(\IoAgent{})=5p$. By our lemma, we can tile the integrated area with self-integrated proper fragments, and because each self-integrated proper fragment contains at least one type-1 cell and one type-2 cell, there are at most $p$ much fragments. Thus, since each self-integrated proper fragment has an area of at most 5, our total integrated area is at most $5p$. But note that $5p$ is achievable as well: since $p\le T$, we simply place $p$ X-pentominos on the board, each with a type-2 cell in the center surrounded by type-1 cells.

Next, we prove that for $p\ge U$, we have $\max(\IoAgent{})=n$; or in other words, it's possible to achieve a fully integrated board. To prove this, it suffices to show that for any $p\in [U, \frac{ab}{2}]$, it's possible to tile the grid with $p$ proper fragments; this is since that if we can tile the grid with $p$ proper fragments, we can simply place one type-1 agent in each fragment, and make the rest of the cells type-2. But note that 

Finally, we place bounds on $T$ and $U$.  Note that X-pentominos tile the plane, so we simply place the board on a plane tiled by X-pentominos. Then, if we consider the set of all X-pentominos whose center lies within the larger $a+2\times b+2$ board surrounding our $a\times b$ board, we see that the union of this set covers every cell on the board. Thus, if we "push up" each X-pentomino center just outside the board as shown in the diagram [insert diagram], we'll have a fragment tiling of the entire board. Hence, we have that $U\le \frac{(a+2)(b+2)}{5}$. 

For $k\in (T, U)$: we can use dynamic programming combined with breadth-first search for an $O(mn)$ algorithm %not sure if this works yet; I have to work out the details

\subsection*{Proof for NP-completeness of IM-IoA}
%I randomly thought of this while trying to figure out how to solve the problem for grids; it seems to be much simpler than the proof in citation 

We can show that IM-IoA is a reduction from finding the cardinality of a minimal dominating set, a well-known NP-hard problem. To do this, first we define a $k$-covering of a graph to be a placement $\mc{P}$ of agents with $|\mc{A}_1|=k$ and $|\mc{A}_2|=n-k$, such that $\IoAgent{}(\mc{P})=n$. We define a graph to be $k$-coverable if there exists a $k$-covering. Now, note that given a minimal dominating set $S$, if we let $\mc{V}_1=S$ and $\mc{V}_2=\mc{V} \backslash \mc{V}_1$, then we will have each type-2 node adjacent to a type-1 node. In addition, no type-1 agent is segregated; this is since if some node $x\in S$ is only connected to other nodes in $S$, then $S$ will still be a dominating set even if we remove $x$, contradicting the minimality of $|S|$. Thus, if the minimum dominating set of a graph has size $k$, then the graph is also $k$-coverable; also, it is clear that in a $k$-covering of a graph, $\mc{A}_1$ is a dominating set. Hence, the cardinality of the minimum dominating set is the first $k$ for which $G$ is $k$-coverable, which can be found by solving IM-IoA on all $k\in [1, n]$. So if IM-IoA is easy, then so is finding the cardinality of the minimum domating set, which is a contradiction. We have thus completed our reduction and proved IM-IoA is NP-hard.

Obviously IM-IoA can be verified in P using a simple DFS, so thus it is NP-complete as well.

\subsubsection*{Running time Improvement (THIS DOES NOT WORK)} 

In the naive implementation of the incremental improvement algorithm where we use DFS to check whether $\IoAgent{}(\mc{P}')>\IoAgent{}(\mc{P})$, we have a runtime of $O(n^4)$. However, by using memoization, we can reduce our total runtime to $O(n^2\log n)$.

To do this, for each agent $a$, let $N_1(a)$ be the number of type-1 neighbors of $a$, let $N_2(a)$ be the number of type-2 neighbors of $a$, let $SN(a)$ be the number of segregated neighbors of $a$, and let $IN(a)$ be the number of integrated neighbors of $a$. In addition, we define a 1-integrated agent to be an integrated agent who has exactly one neighbor of the opposite type; then, for each agent $a$, we let $IN1_1(a)$ denote the number of type-1 1-integrated neighbors of $a$, and let $IN1_2(a)$ denote the number of type-2 1-integrated neighbors of $a$. Note that if we know $N_1(a), N_2(a)$ for all agents $a$, then for a given agent $x$, we can compute $SN(x)$, $IN1_1(x)$, and $IN1_2(x)$ in $O(\deg a)=O(n)$.

Now, note that we can view swapping two agents as simply flipping each of their types. In other words, if $u$ is a type-1 agent and $v$ is a type-2 agent, then swapping $u$ and $v$ is equivalent to flipping $u$ to type-2, followed by flipping $v$ to type-1. So for all agents $a$, let $f(a)$ be $\Delta \IoAgent{}$ when $a$ is flipped.

For an agent $a$, note that if we flip $a$, then each segregated neighbor of $a$ will become integrated, increasing $\IoAgent{}$ by $1$. On the other hand, each opposite-type 1-integrated neighbor of $a$ will become segregated, decreasing $\IoAgent{}$ by 1. Additionally, if $a$ is initially segregated, then flipping $a$ will make $a$ integrated, increasing $\IoAgent{}$ by 1; if $a$ is initially partly integrated (i.e. integrated but with at least one same-type neighbor), then $a$ will still be integrated when it flips, causing no change to $\IoAgent{}$; if $a$ is initially fully integrated (i.e. integrated but without any opposite-type neighbors), then $a$ will become segregated when it flips, decreasing $\IoAgent{}$ by 1. Thus, we have that when we flip $a$, $f(a)=SN(a)-IN1_{3-t}(a)+IS(a)$, where $t$ is the type of $a$ and $IS(a)$ is the "integration state" of $a$ (in particular, $IS(a)=1$ if $a$ is segregated, $IS(a)=0$ if $a$ is partly integrated, and $IS(a)=-1$ if $a$ is fully integrated).

Now, for all pairs $(u, v)$ for which $u\in \mc{A}_1$ and $v\in \mc{A}_2$, let $D(u, v)$ be $\Delta \IoAgent{}$ upon swapping $u, v$. Note that if $u, v$ are not neighbors, we simply have $D(u, v)=f(u)+f(v)$. If $u, v$ are neighbors, to get $D(u, v)$ we first take $f(u)+f(v)$, then add 1 if $u$ is 1-integrated, then add 1 again if $v$ is 1-integrated. So we for any pair $(u, v)$, we can compute $D(u, v)$ in $O(1)$. So at the beginning, we compute $N_1(a), N_2(a), SN(a), IN1_1(a), IN1_2(a)$ in a total of $O(n^2)$ time; then, we compute $D(u, v)$ for all pairs $(u\in \mc{A}_1, v\in\mc{A}_2)$, in a total of $O(n^2)$ time. For our algorithm, we just make a sorted set consisting of all valid triples $(u, v, D(u, v))$, sorted by $D(u, v)$, which takes $O(n^2\log n)$; each step, we take the pair $(u\in \mc{A}_1, v\in \mc{A}_2)$ with the largest $D(u, v)$, flip $u$ and $v$, and update $D(u, x)$ for all $x\in \mc{A}_2$ and update $D(u, y)$ for all $y\in \mc{A}_1$. These updates take $O(n\log n)$ time, and have a maximum of $n$ steps, so our final time complexity is $O(n^2\log n)$.
